# Supplementary material for: A Mountaineering Strategy to Excited States: Highly-Accurate Oscillator Strengths and Dipole Moments of Small Molecules
Source: arXiv:2011.08509 source file (2020-11-17)
Supplement: Supplementary file 1 [file Prop-SI.pdf]

# A Mountaineering Strategy to Excited States: Highly-Accurate Oscillator Strengths and Dipole Moments of Small Molecules Supporting Information

Amara Chrayteh,[†] Aymeric Blondel,[†] Pierre-François Loos,[‡] and Denis Jacquemin[*,†]

†*Université de Nantes, CNRS, CEISAM UMR 6230, F-44000 Nantes, France*

‡*Laboratoire de Chimie et Physique Quantiques, Université de Toulouse, CNRS, UPS, France*

E-mail: Denis.Jacquemin@univ-nantes.fr

# S1 Comparison between EOM and LR $f$

Table S1: Comparison between the EOM and LR $f$ obtained at the CCSD/*aug*-cc-pVTZ level with various codes. Length gauge data are reported.

| | | LR-CCSD | | | EOM-CCSD | |
|---|---|---|---|---|---|---|
| Molecule | State | MRCC | Dalton | Gaussian | $e^T$ | Gaussian |
| BH | $^1\Pi$ | 0.050 | 0.050 | 0.050 | 0.050 | 0.051 |
| HCl | $^1\Pi$ | 0.056 | 0.056 | 0.056 | 0.055 | 0.055 |
| $H_2O$ | $^1B_1$ | 0.053 | 0.053 | 0.054 | 0.054 | 0.054 |
| | $^1A_1$ | 0.098 | 0.099 | 0.098 | 0.099 | 0.099 |
| $H_2S$ | $^1B_1$ | 0.064 | 0.064 | 0.064 | 0.063 | 0.063 |
| BF | $^1\Pi$ | 0.475 | 0.475 | 0.475 | 0.482 | 0.482 |
| CO | $^1\Pi$ | 0.161 | 0.161 | 0.161 | 0.164 | 0.164 |
| | $^1\Sigma^+$ | 0.008 | 0.008 | 0.008 | 0.008 | 0.008 |
| | $^1\Sigma^+$ | 0.208 | 0.208 | 0.208 | 0.209 | 0.209 |
| | $^1\Pi$ | 0.115 | 0.115 | 0.115 | 0.115 | 0.115 |
| $N_2$ | $^1\Pi_u$ | 0.439 | 0.439 | 0.439 | 0.446 | 0.446 |
| | $^1\Sigma_u^+$ | 0.263 | 0.263 | 0.263 | 0.265 | 0.265 |
| | $^1\Pi_u$ | 0.053 | 0.053 | 0.053 | 0.056 | 0.056 |
| | $^1\Pi_u$ | 0.136 | 0.136 | 0.136 | 0.136 | 0.136 |
| Ethylene | $B_{3u}$ | 0.078 | 0.078 | 0.078 | 0.079 | 0.079 |
| | $B_{1u}$ | 0.362 | 0.361 | 0.362 | 0.370 | 0.370 |
| Formaldehyde | $B_2$ | 0.018 | 0.018 | 0.018 | 0.018 | 0.018 |
| | $B_2$ | 0.040 | 0.040 | 0.040 | 0.040 | 0.040 |
| | $A_1$ | 0.054 | 0.054 | 0.054 | 0.054 | 0.054 |
| | $A_1$ | 0.139 | 0.140 | 0.139 | 0.143 | 0.143 |
| Thioformaldehyde | $B_2$ | 0.014 | 0.014 | 0.014 | 0.014 | 0.014 |
| | $A_1$ | 0.206 | 0.206 | 0.206 | 0.216 | 0.216 |
| Fluorocarbene | $^1A''$ | 0.006 | 0.006 | 0.006 | 0.007 | 0.007 |
| Silylidene | $B_2$ | 0.036 | 0.036 | 0.036 | 0.037 | 0.037 |

# S2 Impact of the FC approximation for BH

Table S2: Comparison between the properties of BH obtained with *aug*-cc-pVTZ (FC) *aug*-cc-pCVTZ (Full correlation). The dipole moments are in D.

| | *aug*-cc-pVTZ, frozen-core | | | | *aug*-cc-pCVTZ, full | | | |
|---|---|---|---|---|---|---|---|---|
| | $^1\Sigma^+$ | $^1\Pi$ (Val) | | | $^1\Sigma^+$ | $^1\Pi$ (Val) | | |
| Method | $\mu^{\text{GS}}$ | $f$ | $\mu^{\text{ES}}_{\text{vert}}$ | $\mu^{\text{ES}}_{\text{adia}}$ | $\mu^{\text{GS}}$ | $f$ | $\mu^{\text{ES}}_{\text{vert}}$ | $\mu^{\text{ES}}_{\text{adia}}$ |
| CCSD | 1.433 | 0.050 | 0.550 | 0.534 | 1.441 | 0.050 | 0.554 | 0.538 |
| CCSDT | 1.410 | 0.048 | 0.558 | 0.541 | 1.411 | 0.048 | 0.556 | 0.539 |
| CCSDTQ | 1.409 | 0.048 | 0.559 | 0.542 | 1.410 | 0.047 | 0.557 | 0.540 |

# S3 Extra data obtained on ES geometries

## S3.1 BH

Table S3: Vertical transition energies $\Delta E_{\text{vert}}$ (in eV) determined on the ES geometry of BH. The dipole values are given in Table 1 in the main text.

| Basis | Method | $^1\Pi$ (Val) $\Delta E_{\text{vert}}$ |
|---|---|---|
| *aug*-cc-pVDZ | CCSD | 2.966 |
| | CCSDT | 2.943 |
| | CCSDTQ | 2.945 |
| | CCSDTQP | 2.945 |
| *aug*-cc-pVTZ | CCSD | 2.924 |
| | CCSDT | 2.897 |
| | CCSDTQ | 2.898 |
| *aug*-cc-pVQZ | CCSD | 2.914 |
| | CCSDT | 2.887 |
| *aug*-cc-pV5Z | CCSD | 2.911 |
| d-*aug*-cc-pVDZ | CCSD | 2.965 |
| | CCSDT | 2.943 |
| d-*aug*-cc-pVTZ | CCSD | 2.923 |
| | CCSDT | 2.897 |
| d-*aug*-cc-pVQZ | CCSD | 2.914 |
| | CCSDT | 2.886 |

## S3.2 CO

Table S4: Vertical transition energies $\Delta E_{\text{vert}}$ (in eV), oscillator strength $f$, and excited-state dipole moments $\mu^{\text{ES}}$ (in D) determined on the ES geometries of CO. See also Table 5 in the main text.

| | | $^1\Pi(\text{Val}, n \to \pi^\star)$ | | | $^1\Sigma^+$(Ryd) | | | $^1\Sigma^+$(Ryd) | | |
|---|---|---|---|---|---|---|---|---|---|---|
| Basis | Method | $\Delta E_{\text{vert}}$ | $f$ | $\mu^{\text{ES}}$ | $\Delta E_{\text{vert}}$ | $f$ | $\mu^{\text{ES}}$ | $\Delta E_{\text{vert}}$ | $f$ | $\mu^{\text{ES}}$ |
| *aug*-cc-pVDZ | CCSD | 7.671 | 0.088 | -0.438 | 11.164 | 0.002 | -4.181 | 11.701 | 0.244 | 6.385 |
| | CCSDT | 7.598 | 0.094 | -0.331 | 10.940 | 0.000 | -4.558 | 11.513 | 0.236 | 6.750 |
| | CCSDTQ | 7.590 | 0.095 | -0.317 | 10.922 | 0.000 | -4.609 | 11.504 | 0.235 | 6.817 |
| | CCSDTQP | 7.588 | 0.096 | -0.312 | 10.915 | 0.001 | -4.628 | 11.501 | 0.235 | 6.840 |
| *aug*-cc-pVTZ | CCSD | 7.565 | 0.085 | -0.478 | 11.216 | 0.007 | -3.421 | 11.740 | 0.205 | 5.660 |
| | CCSDT | 7.493 | 0.089 | -0.358 | 10.983 | 0.003 | -3.932 | 11.533 | 0.200 | 6.147 |
| | CCSDTQ | 7.485 | 0.090 | -0.344 | 10.960 | 0.003 | -4.031 | 11.517 | 0.199 | 6.254 |
| *aug*-cc-pVQZ | CCSD | 7.554 | 0.085 | -0.511 | 11.184 | 0.009 | -2.829 | 11.722 | 0.180 | 5.150 |
| | CCSDT | 7.481 | 0.088 | -0.385 | 10.949 | 0.005 | -3.383 | 11.507 | 0.177 | 5.666 |
| *aug*-cc-pV5Z | CCSD | 7.551 | 0.085 | -0.523 | 11.126 | 0.011 | -2.106 | 11.680 | 0.158 | 4.656 |
| d-*aug*-cc-pVDZ | CCSD | 7.666 | 0.088 | -0.442 | 10.786 | 0.008 | -1.486 | 11.382 | 0.132 | 3.530 |
| | CCSDT | 7.591 | 0.093 | -0.334 | 10.563 | 0.005 | -2.001 | 11.167 | 0.119 | 3.954 |
| d-*aug*-cc-pVTZ | CCSD | 7.563 | 0.085 | -0.483 | 10.953 | 0.010 | -1.358 | 11.555 | 0.132 | 3.845 |
| | CCSDT | 7.491 | 0.088 | -0.364 | 10.721 | 0.006 | -1.874 | 11.332 | 0.129 | 4.244 |
| d-*aug*-cc-pVQZ | CCSD | 7.553 | 0.085 | -0.513 | 11.002 | 0.010 | -1.320 | 11.606 | 0.132 | 3.978 |
| | CCSDT | 7.480 | 0.088 | -0.389 | 10.796 | 0.007 | -1.830 | 11.380 | 0.129 | 4.366 |

## S3.3 Formaldehyde

Table S5: Vertical transition energies $\Delta E_{\mathrm{vert}}$ (in eV), oscillator strength $f$, and excited-state dipole moments $\mu^{\mathrm{ES}}$ (in D) determined on the ES geometries of formaldehyde. See also Table 8 in the main text.

| | | $^1A''(\mathrm{Val}, n \to \pi^\star)$ | | $^1B_2(\mathrm{Ryd}, n \to 3s)$ | | |
|---|---|---|---|---|---|---|
| Basis | Method | $\Delta E_{\mathrm{vert}}$ | $\mu^{\mathrm{ES}}$ | $\Delta E_{\mathrm{vert}}$ | $f$ | $\mu^{\mathrm{ES}}$ |
| 6-31+G(d) | CCSD | 2.916 | 1.870 | 7.145 | 0.024 | -0.479 |
| | CCSDT | 2.850 | 1.790 | 7.137 | 0.028 | -0.990 |
| | CCSDTQ | 2.862 | 1.751 | 7.184 | 0.027 | -0.906 |
| | CCSDTQP | 2.863 | | 7.192 | 0.027 | -0.885 |
| *aug*-cc-pVDZ | CCSD | 2.924 | 1.602 | 6.935 | 0.025 | -1.634 |
| | CCSDT | 2.844 | 1.524 | 6.927 | 0.028 | -1.976 |
| | CCSDTQ | 2.855 | 1.486 | 6.978 | 0.028 | -1.932 |
| *aug*-cc-pVTZ | CCSD | 2.928 | 1.620 | 7.120 | 0.026 | -1.476 |
| | CCSDT | 2.819 | 1.534 | 7.049 | 0.028 | -1.873 |
| *aug*-cc-pVQZ | CCSD | 2.943 | 1.635 | 7.184 | 0.026 | -1.406 |
| d-*aug*-cc-pVDZ | CCSD | 2.921 | 1.596 | 6.921 | 0.023 | -1.410 |
| | CCSDT | 2.840 | 1.518 | 6.913 | 0.026 | -1.803 |
| d-*aug*-cc-pVTZ | CCSD | 2.927 | 1.619 | 7.114 | 0.025 | -1.309 |
| | CCSDT | 2.818 | 1.533 | 7.043 | 0.027 | -1.743 |
| d-*aug*-cc-pVQZ | CCSD | 2.943 | 1.636 | 7.181 | 0.025 | -1.299 |

## S3.4 Thioformaldehyde

Table S6: Vertical transition energies $\Delta E_{\text{vert}}$ (in eV), oscillator strength $f$, and excited-state dipole moments $\mu^{\text{ES}}$ (in D) determined on the ES geometries of thioformaldehyde. See also Table 9 in the main text.

| | | $^1A_2(\text{Val}, n \rightarrow \pi^\star)$ | | $^1B_2(\text{Ryd}, n \rightarrow 4s)$ | | |
|---|---|---|---|---|---|---|
| Basis | Method | $\Delta E_{\text{vert}}$ | $\mu^{\text{ES}}$ | $\Delta E_{\text{vert}}$ | $f$ | $\mu^{\text{ES}}$ |
| 6-31+G(d) | CCSD | 2.040 | 0.968 | 5.886 | 0.018 | -3.070 |
| | CCSDT | 1.964 | 0.990 | 5.822 | 0.017 | -3.257 |
| | CCSDTQ | 1.967 | 0.947 | 5.836 | 0.017 | -3.253 |
| | CCSDTQP | 1.968 | 0.943 | 5.839 | 0.018 | -3.252 |
| *aug*-cc-pVDZ | CCSD | 2.072 | 0.873 | 5.779 | 0.011 | -3.693 |
| | CCSDT | 1.980 | 0.898 | 5.732 | 0.010 | -3.885 |
| | CCSDTQ | 1.982 | 0.864 | 5.751 | 0.010 | -3.885 |
| *aug*-cc-pVTZ | CCSD | 2.050 | 0.870 | 5.909 | 0.013 | -3.149 |
| | CCSDT | 1.943 | 0.890 | 5.835 | 0.011 | -3.422 |
| *aug*-cc-pVQZ | CCSD | 2.059 | 0.890 | 5.957 | 0.013 | -2.944 |
| d-*aug*-cc-pVDZ | CCSD | 2.070 | 0.877 | 5.745 | 0.014 | -3.055 |
| | CCSDT | 1.979 | 0.901 | 5.698 | 0.013 | -3.281 |
| d-*aug*-cc-pVTZ | CCSD | 2.050 | 0.872 | 5.898 | 0.014 | -2.847 |
| | CCSDT | 1.943 | 0.892 | 5.824 | 0.012 | -3.154 |
| d-*aug*-cc-pVQZ | CCSD | 2.059 | 0.892 | 5.951 | 0.013 | -2.794 |

## S3.5 Nitroxyl

Table S7: Vertical transition energies $\Delta E_{\mathrm{vert}}$ (in eV) determined on the ES geometry of HNO. The dipole values are given in Table 10 in the main text.

| Basis | Method | $^1A''$ (Val) $\Delta E_{\mathrm{vert}}$ |
|---|---|---|
| 6-31+G(d) | CCSD | 1.614 |
| | CCSDT | 1.611 |
| | CCSDTQ | 1.614 |
| | CCSDTQP | 1.614 |
| *aug*-cc-pVDZ | CCSD | 1.587 |
| | CCSDT | 1.577 |
| | CCSDTQ | 1.580 |
| *aug*-cc-pVTZ | CCSD | 1.564 |
| | CCSDT | 1.548 |
| *aug*-cc-pVQZ | CCSD | 1.562 |
| d-*aug*-cc-pVDZ | CCSD | 1.586 |
| | CCSDT | 1.576 |
| d-*aug*-cc-pVTZ | CCSD | 1.564 |
| | CCSDT | 1.547 |
| d-*aug*-cc-pVQZ | CCSD | 1.562 |

# S4 Cartesian coordinates

Below, we provide the Cartesian coordinates of the compounds investigated in this study. These are given in atomic units (bohr) and they have been obtained at the CC3(full)/*aug*-cc-pVTZ level of theory.

### S4.0.1 BH

Ground state

| | | | |
|---|---|---|---|
| B | 0.00000000 | 0.00000000 | 0.00000000 |
| H | 0.00000000 | 0.00000000 | 2.31089693 |

Excited state

| | | | |
|---|---|---|---|
| B | 0.00000000 | 0.00000000 | 0.00000000 |
| H | 0.00000000 | 0.00000000 | 2.27596436 |

## S4.1 Hydrogen chloride (HCl)

| | | | |
|---|---|---|---|
| H | 0.00000000 | 0.00000000 | 2.38483140 |
| Cl | 0.00000000 | 0.00000000 | -0.02489783 |

## S4.2 Water ($H_2O$)

| | | | |
|---|---|---|---|
| O | 0.00000000 | 0.00000000 | -0.13209669 |
| H | 0.00000000 | 1.43152878 | 0.97970006 |
| H | 0.00000000 | -1.43152878 | 0.97970006 |

## S4.3 Hydrogen sulfide ($H_2S$)

| | | | |
|---|---|---|---|
| S | 0.00000000 | 0.00000000 | -0.50365086 |
| H | 0.00000000 | 1.81828105 | 1.25212288 |
| H | 0.00000000 | -1.81828105 | 1.25212288 |

### S4.3.1 BF

| | | | |
|---|---|---|---|
| B | 0.00000000 | 0.00000000 | 0.00000000 |
| F | 0.00000000 | 0.00000000 | 2.39729626 |

### S4.3.2 Carbon monoxide (CO)

Ground state

| | | | |
|---|---|---|---|
| C | 0.00000000 | 0.00000000 | -1.24942055 |
| O | 0.00000000 | 0.00000000 | 0.89266692 |

$S_1$, $^1\Pi(\mathrm{Val}, n \to \pi^\star)$

| | | | |
|---|---|---|---|
| C | 0.00000000 | 0.00000000 | -1.34361664 |
| O | 0.00000000 | 0.00000000 | 1.01049741 |

$S_4$, $^1\Sigma^+(\mathrm{Ryd})$

| | | | |
|---|---|---|---|
| C | 0.00000000 | 0.00000000 | -1.21900157 |
| O | 0.00000000 | 0.00000000 | 0.91332258 |

$S_5$, $^1\Sigma^+(\mathrm{Ryd})$

| | | | |
|---|---|---|---|
| C | 0.00000000 | 0.00000000 | -1.21767685 |
| O | 0.00000000 | 0.00000000 | 0.91199786 |

## S4.4 Dinitrogen ($N_2$)

| | | | |
|---|---|---|---|
| N | 0.00000000 | 0.00000000 | 1.04008632 |
| N | 0.00000000 | 0.00000000 | -1.04008632 |

## S4.5 Ethylene ($C_2H_2$)

| | | | |
|---|---|---|---|
| C | 0.00000000 | 1.26026583 | 0.00000000 |
| C | 0.00000000 | -1.26026583 | 0.00000000 |
| H | 0.00000000 | 2.32345976 | 1.74287672 |
| H | 0.00000000 | -2.32345976 | 1.74287672 |
| H | 0.00000000 | 2.32345976 | -1.74287672 |
| H | 0.00000000 | -2.32345976 | -1.74287672 |

### S4.5.1 Formaldehyde ($CH_2O$)

Ground state

| | | | |
|---|---|---|---|
| C | 0.00000000 | 0.00000000 | 1.13947666 |
| O | 0.00000000 | 0.00000000 | -1.14402883 |
| H | 0.00000000 | 1.76627623 | 2.23398653 |
| H | 0.00000000 | -1.76627623 | 2.23398653 |

$S_1$, $^1A_2(\mathrm{Val}, n \rightarrow \pi^\star)$

| | | | |
|---|---|---|---|
| C | -0.09942705 | 0.00000000 | 1.27071070 |
| O | 0.01987299 | 0.00000000 | -1.23280536 |
| H | 0.42778855 | 1.76729629 | 2.18470884 |
| H | 0.42778855 | -1.76729629 | 2.18470884 |

$S_2$, $^1B_2(\mathrm{Ryd}, n \rightarrow 3s)$

| | | | |
|---|---|---|---|
| C | 0.00000000 | 0.00000000 | 1.00526570 |
| O | 0.00000000 | 0.00000000 | -1.26661095 |
| H | 0.00000000 | 1.88258795 | 2.02322767 |
| H | 0.00000000 | -1.88258795 | 2.02322767 |

### S4.5.2 Thioformaldehyde ($CH_2S$)

Ground state

| | | | |
|---|---|---|---|
| C | 0.00000000 | 0.00000000 | 2.08677304 |
| S | 0.00000000 | 0.00000000 | -0.97251194 |
| H | 0.00000000 | 1.73657773 | 3.17013507 |
| H | 0.00000000 | -1.73657773 | 3.17013507 |

$S_1$, $^1A_2(\mathrm{Val}, n \rightarrow \pi^\star)$

| | | | |
|---|---|---|---|
| C | 0.00000000 | 0.00000000 | 2.20256705 |
| S | 0.00000000 | 0.00000000 | -1.02717172 |
| H | 0.00000000 | 1.76634191 | 3.21909384 |
| H | 0.00000000 | -1.76634191 | 3.21909384 |

$S_2$, $^1B_2(\mathrm{Ryd}, n \rightarrow 4s)$

| | | | |
|---|---|---|---|
| C | 0.00000000 | 0.00000000 | 2.06792111 |
| S | 0.00000000 | 0.00000000 | -0.96974849 |
| H | 0.00000000 | 1.81570729 | 3.09198823 |
| H | 0.00000000 | -1.81570729 | 3.09198823 |

### S4.5.3 Nitroxyl (HNO)

Ground state

| | | | |
|---|---|---|---|
| O | 0.21099695 | 0.00000000 | 2.15462460 |
| N | -0.44776863 | 0.00000000 | -0.03589263 |
| H | 1.18163475 | 0.00000000 | -1.17386890 |

Excited state

| | | | |
|---|---|---|---|
| O | 0.11093762 | 0.00000000 | -1.22472054 |
| N | 0.11245127 | 0.00000000 | 1.11281929 |
| H | -1.64569693 | 0.00000000 | 1.96953983 |

### S4.5.4 Fluorocarbene (HCF)

| | | | |
|---|---|---|---|
| C | -0.13561085 | 0.00000000 | 1.20394474 |
| F | 1.85493976 | 0.00000000 | -0.27610752 |
| H | -1.71932891 | 0.00000000 | -0.18206846 |

### S4.5.5 Silylidene ($H_2CSi$)

| | | | |
|---|---|---|---|
| C | 0.00000000 | 0.00000000 | -2.09539928 |
| Si | 0.00000000 | 0.00000000 | 1.14992930 |
| H | 0.00000000 | 1.70929524 | -3.22894481 |
| H | 0.00000000 | -1.70929524 | -3.22894481 |
